# Supplementary material for: Electron-phonon-dominated charge-density-wave fluctuations in TiSe$_2$ accessed by ultrafast nonequilibrium dynamics
Source: arXiv:2507.12430 source file (2026-01-16)
Supplement: Supplementary file 1 [file Supplement.pdf]

**Supplemental Material for:**  
**Electron-phonon-dominated charge-density-wave fluctuations in  $\text{TiSe}_2$  accessed by**  
**ultrafast nonequilibrium dynamics**

Sotirios Fragkos,<sup>1</sup> Hibiki Orio,<sup>2,\*</sup> Nina Giroto Erhardt,<sup>3,4</sup> Akib Javed,<sup>1,5</sup> Sarath Sasi,<sup>6</sup> Quentin Courtade,<sup>1</sup> Muthu P. T. Masilamani,<sup>2</sup> Maximilian Ünzelmann,<sup>2</sup> Florian Diekmann,<sup>7,8</sup> Baptiste Hildebrand,<sup>9</sup> Dominique Descamps,<sup>1</sup> Stéphane Petit,<sup>1</sup> Fabio Boschini,<sup>10</sup> Ján Minár,<sup>6</sup> Yann Mairesse,<sup>1</sup> Friedrich Reinert,<sup>2</sup> Kai Rossnagel,<sup>7,8</sup> Dino Novko,<sup>3,†</sup> Samuel Beaulieu,<sup>1</sup> and Jakub Schusser<sup>2,6,‡</sup>

<sup>1</sup>*Université de Bordeaux - CNRS - CEA, CELIA, UMR5107, F33405 Talence, France*

<sup>2</sup>*Experimentelle Physik VII and Würzburg-Dresden Cluster of Excellence ct.qmat,  
Universität Würzburg, D-97074, Würzburg, Germany*

<sup>3</sup>*Centre for Advanced Laser Techniques, Institute of Physics, 10000 Zagreb, Croatia*

<sup>4</sup>*European Theoretical Spectroscopy Facility, Institute of Condensed Matter and Nanosciences,  
Université catholique de Louvain, Louvain-la-Neuve, Belgium*

<sup>5</sup>*Institut National de la Recherche Scientifique – Énergie Matériaux Télécommunications Varennes, QC J3X 1S2, Canada*

<sup>6</sup>*New Technologies-Research Center, University of West Bohemia, 30614, Pilsen, Czech Republic*

<sup>7</sup>*Ruprecht Haensel Laboratory, Deutsches Elektronen-Synchrotron DESY, D-22607, Hamburg, Germany*

<sup>8</sup>*Institute of Experimental and Applied Physics, Kiel University, D-24098, Kiel, Germany*

<sup>9</sup>*University of Fribourg and Fribourg Centre for Nanomaterials,  
Chemin du Musée 3, CH-1700 Fribourg, Switzerland*

<sup>10</sup>*Advanced Laser Light Source, Institut National de la Recherche Scientifique, Varennes QC J3X 1S2 Canada*

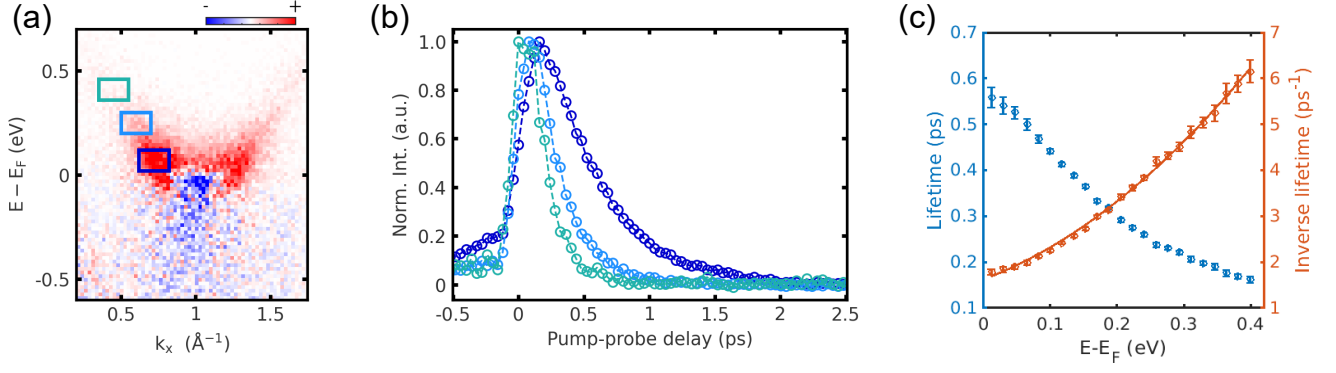

FIG. S1. (a) Differential energy-momentum cut near M with several regions of interest (ROI) boxes. The red and blue intensities denote the contrast between the pre-pump (integrated from -880 fs to -720 fs) and pump-probe overlap (integrated from -80 fs to 80 fs). (b) Intensity dynamics within each ROI, illustrating the faster decay of photoexcited electrons at higher energies. (c) Momentum-integrated electron population lifetime and corresponding inverse lifetime as a function of  $E - E_F$ .

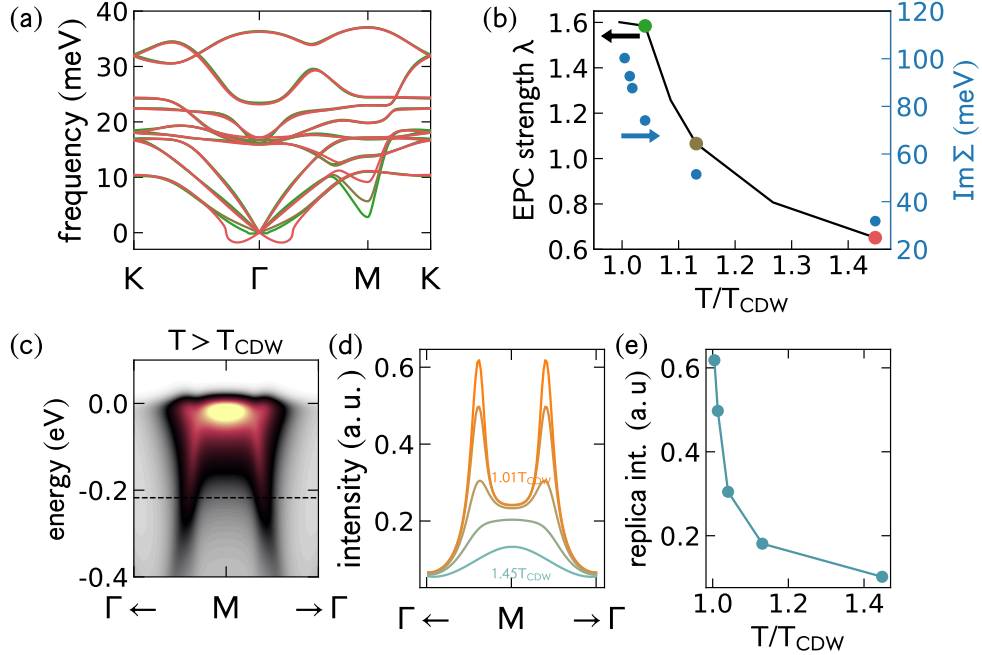

FIG. S2. (a) Phonon band structure of non-distorted TiSe<sub>2</sub> along the high-symmetry points and for several temperatures above the  $T_{\text{CDW}}$ , i.e., for 1150 K, 1300 K, and 1600 K. Note that this is done within the harmonic approximation for which  $T_{\text{CDW}} \approx 1100$  K. Also, note the hardening of the CDW-related acoustic phonon at the M point. (b) The calculated total electron-phonon coupling (EPC) strength  $\lambda$  for each temperature above  $T_{\text{CDW}}$ . The right axis shows the values for the imaginary part of the electron self-energy due to EPC (i.e., electron scattering rate), averaged over the states around the Fermi level. (c) Fluctuating replica at the M point for temperatures above  $T_{\text{CDW}}$  as obtained from the dynamical EPC scatterings. (d) The corresponding intensity of the fluctuating CDW replica coming from dynamical EPC as a function of temperature and along the M point. (e) The intensity of the replica is decreasing as a function of temperature. Note the connection between the hardening of the M acoustic phonon, the weakening of the EPC strength, and quenching of the CDW fluctuating replica as a function of increasing temperature.

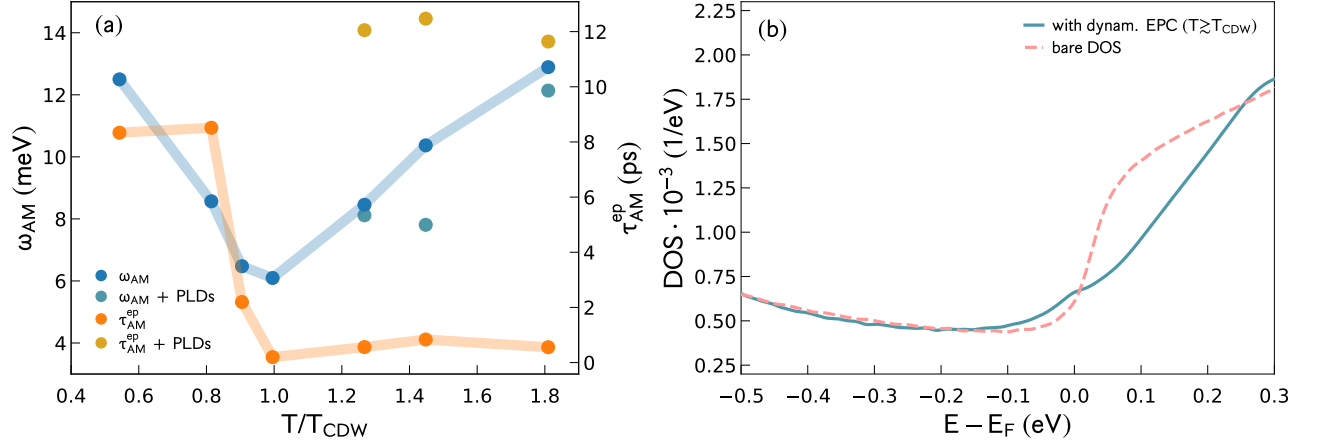

FIG. S3. (a) Frequency (blue) and lifetime (orange) of the CDW amplitude mode calculated from DFPT. We also show the corresponding results where small periodic lattice distortions are introduced also for  $T > T_{CDW}$  to mimic the CDW fluctuations. (b) Density of states for the bare  $\text{TiSe}_2$  electronic structure, as well as when the dynamical electron-phonon scatterings are included for  $T > T_{CDW}$ . The opening of the pseudogap is evident for the latter.

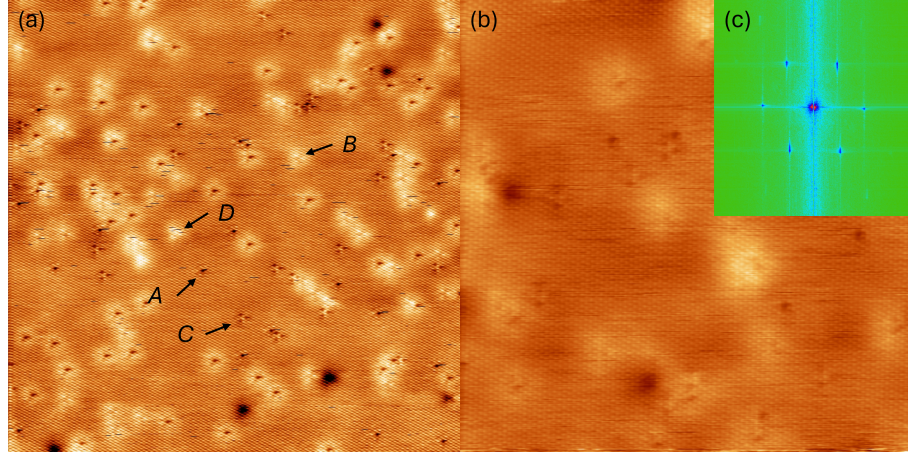

FIG. S4. To characterize the CDW fluctuations dynamics in real space and find the fingerprints of finite fluctuating periodic lattice distortions (PLD), we measured the  $1\text{T-TiSe}_2$  at RT with scanning tunneling microscopy (STM) and observed no visible signatures of the  $2 \times 2$  CDW patches beyond the signal corresponding to the  $1 \times 1$  unit cell charge modulation. This implies that the fluctuations probably occur at timescales below the scanning rate of the STM and further supports our result that the CDW fluctuations in  $\text{TiSe}_2$  are dynamical. Despite that, L and M diffusive peaks at RT were spotted in equilibrium electron diffraction measurements<sup>S1</sup>, as well as in X-ray diffuse scattering<sup>S2,S3</sup>, suggesting the presence of the fluctuating PLD at RT, and possibly the appearance of the corresponding pseudogap<sup>S4</sup>. (a) Atomically resolved empty-states STM image showing native defects ( $60 \times 60 \text{ nm}^2$ ,  $I_t = 1.2 \text{ nA}$ ,  $V_{\text{bias}} = 0.01 \text{ V}$ ). Different defects are labeled A, B, C, D following (PRL<sup>S5</sup>). (b) Atomically resolved filled-states STM image ( $32 \times 32 \text{ nm}^2$ ,  $I_t = 0.1 \text{ nA}$ ,  $V_{\text{bias}} = -0.1 \text{ V}$ ). (c) FFT-amplitude plot from (b) showing no  $2 \times 2$  CDW charge modulation associated spots.

\* [hibiki.orio@uni-wuerzburg.de](mailto:hibiki.orio@uni-wuerzburg.de)

† [dino.novko@gmail.com](mailto:dino.novko@gmail.com)

‡ [schusser@ntc.zcu.cz](mailto:schusser@ntc.zcu.cz)

- [S1] Y. Cheng, A. Zong, J. Li, W. Xia, S. Duan, W. Zhao, Y. Li, F. Qi, J. Wu, L. Zhao, *et al.*, [Nature communications](#) **13**, 963 (2022).
- [S2] K. C. Woo, F. C. Brown, W. L. McMillan, R. J. Miller, M. J. Schaffman, and M. P. Sears, [Phys. Rev. B](#) **14**, 3242 (1976).
- [S3] X. Guo, A. Kogar, J. Henke, F. Flicker, F. de Juan, S. X. L. Sun, I. Khayr, Y. Peng, S. Lee, M. J. Krogstad, S. Rosenkranz, R. Osborn, J. P. C. Ruff, D. B. Lioi, G. Karapetrov, D. J. Campbell, J. Paglione, J. van Wezel, T. C. Chiang, and P. Abbamonte, [arXiv](#) , 2501.09968 (2025).
- [S4] Y. Miyahara, H. Bando, and H. Ozaki, [Journal of Physics: Condensed Matter](#) **7**, 2553 (1995).
- [S5] B. Hildebrand, C. Didiot, A. M. Novello, G. Monney, A. Scarfato, A. Ubaldini, H. Berger, D. R. Bowler, C. Renner, and P. Aebi, [Phys. Rev. Lett.](#) **112**, 197001 (2014).
